# Supplementary material for: Training-Free Style and Content Transfer by Leveraging U-Net Skip Connections in Stable Diffusion
Source: arXiv:2501.14524 source file (2025-04-04)
Supplement: Supplementary file 1 [file X_suppl.tex]

\clearpage
\setcounter{page}{1}
\maketitlesupplementary

In this Supplementary Material, we present the following sections to support the findings of the main paper:
\begin{itemize}
    \item \textbf{effect of different versions of Stable Diffusion} where we show the impact of SkipInject on Stable Diffusion 1.4, 1.5, 2, 2.1, Turbo, and XL and find that 1.4-1.5 and XL share a similar representation split that differs from all 2.* versions treated in the paper.
    %\item \textbf{Properties of the embeddings of skip l=4} where we plot the embeddings of the skip connections to understand their structure and properties.
    \item \textbf{ablation studies on the hyperparameters} where we show our model's qualitative and quantitative results on different combinations of the hyperparameters both for style transfer and text-guided image editing.
    \item \textbf{examples on Turbo} where we show examples generated using SkipInject on Turbo, showing extremely promising results on one-step inference.
    
\end{itemize}

\section{Effect of different versions of Stable Diffusion}
\label{sec:versions}
\begin{figure}[h]
\centering
\includegraphics[width=0.5\textwidth]{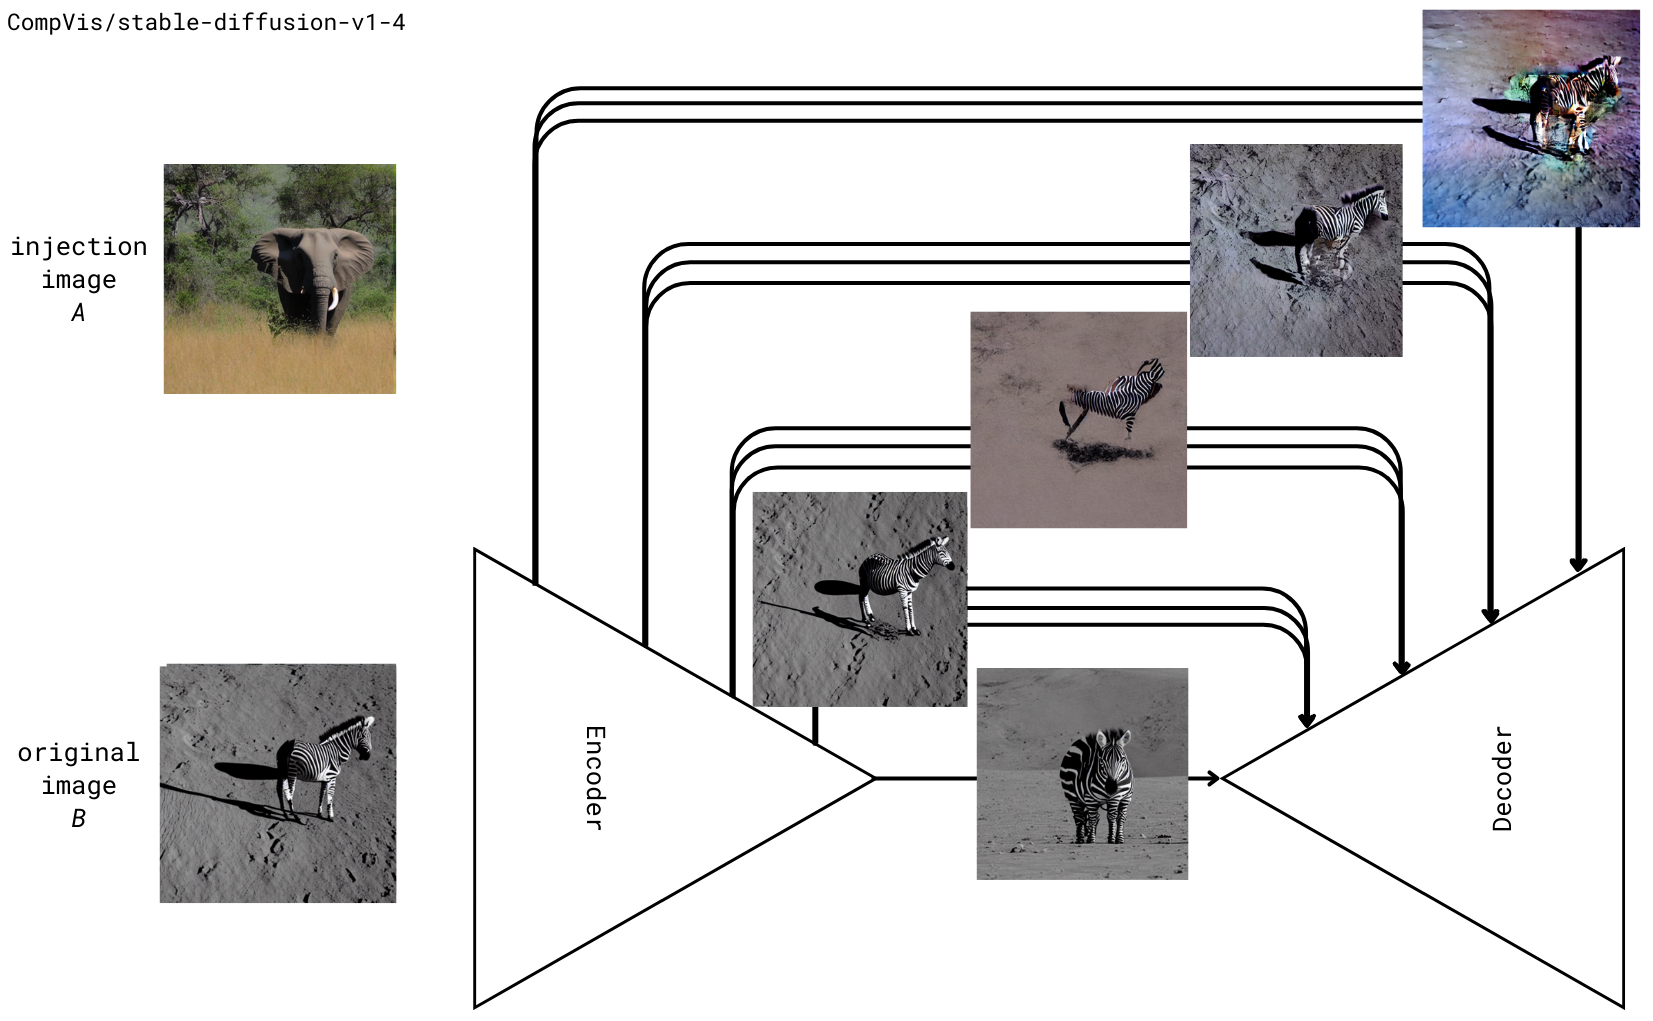}
\includegraphics[width=0.5\textwidth]{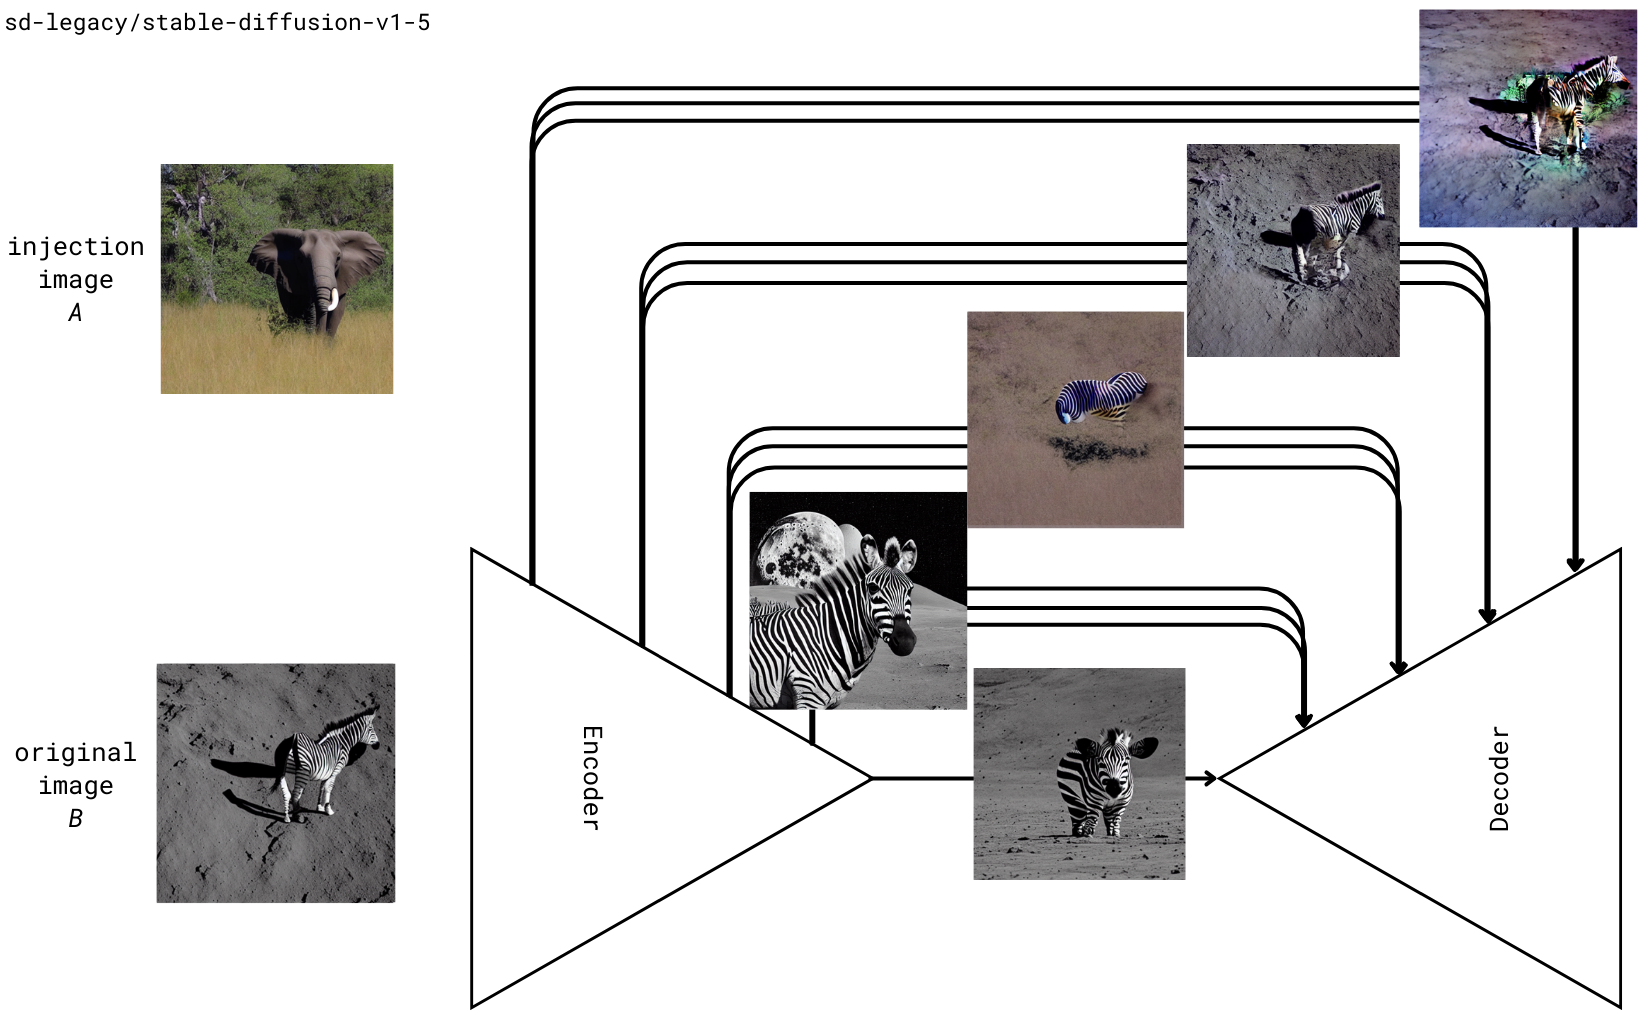}
\caption{Visualization of SkipInject effect on v1.4 and v1.5. As visible in the figure, the effect of the second group of skip connections is now split between the \textit{h-space}, carrying the content of the foreground, and the second group of skips, determining the content of the background without structure.}
\label{fig:versions1}
\end{figure}

The main paper focuses on Stable Diffusion v2.0. In this Supplementary Material section, we investigate whether the phenomenon identified on Stable Diffusion v2.0 extends to other versions of UNet-based Stable Diffusions and whether the previously observed importance of the \textit{h-space}, presented in the Introduction, can be found in other versions. To understand whether the models form different representations, we carry out the same experiment on different versions of Stable Diffusion. We find that Stable Diffusion 2 and 2.1 behave similarly, as well as the Turbo version of 2.1, while Stable Diffusion 1.4, 1.5, and XL show a more profound impact of the \textit{h-space}, shown in \cref{fig:versions1}. 

\begin{figure}[h]
\centering
\includegraphics[width=0.5\textwidth]{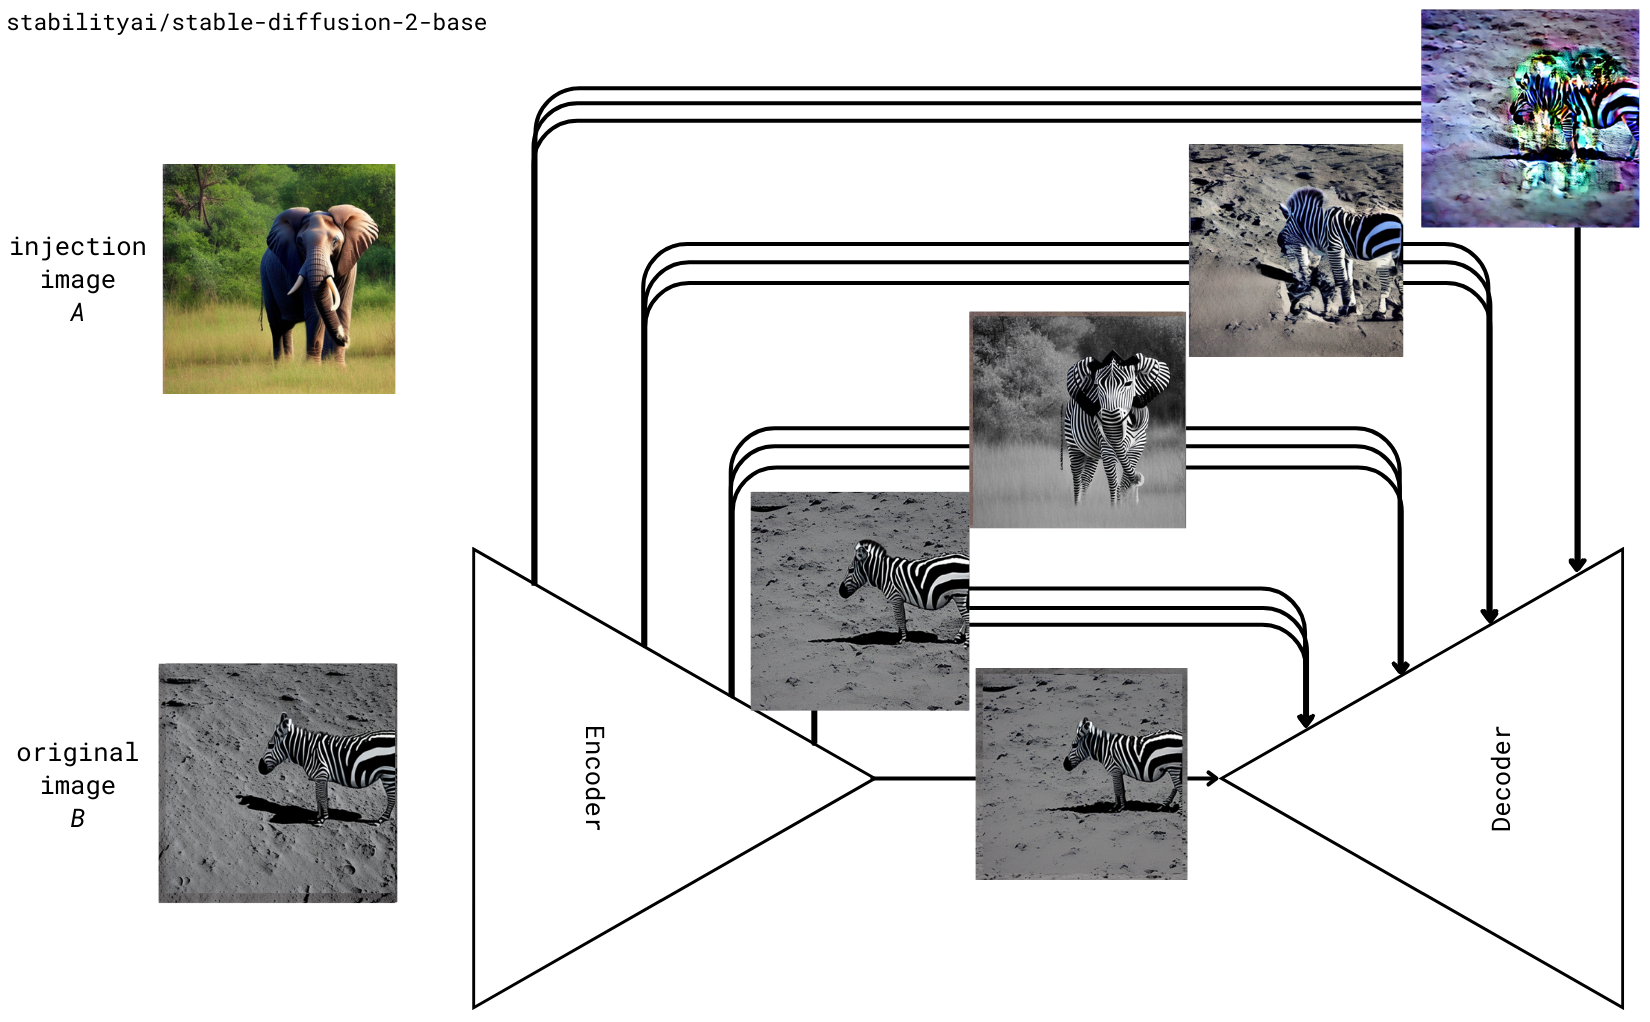}
\includegraphics[width=0.5\textwidth]{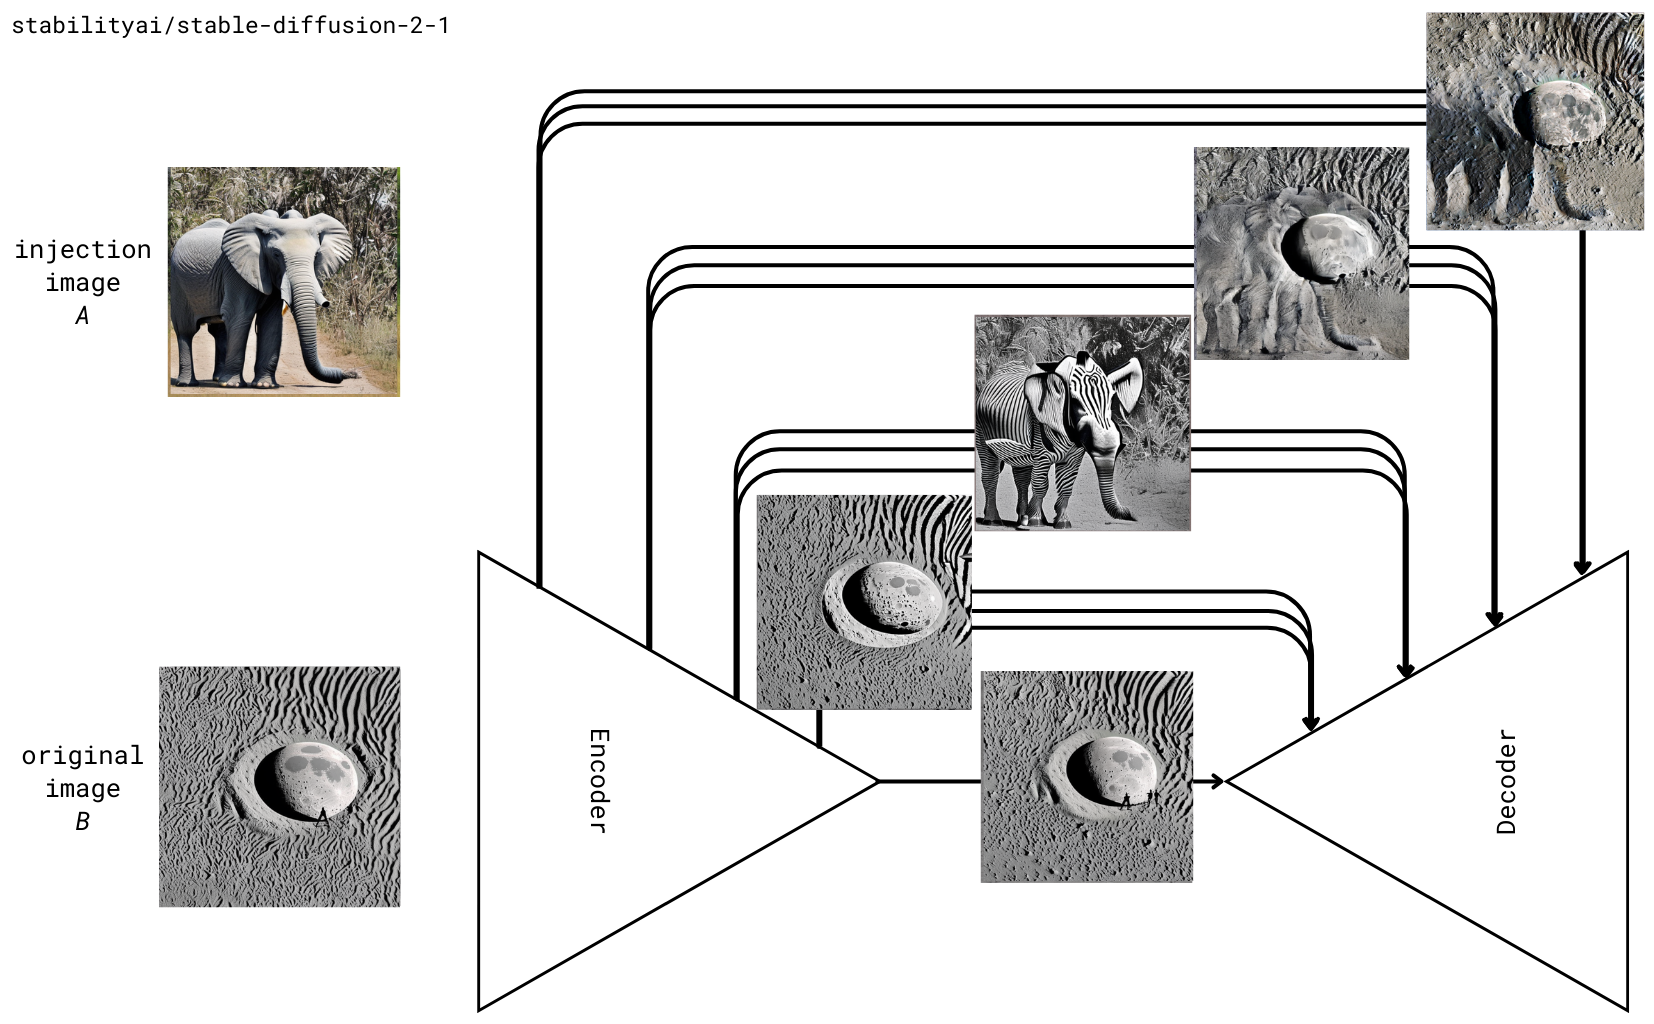}
\includegraphics[width=0.5\textwidth]{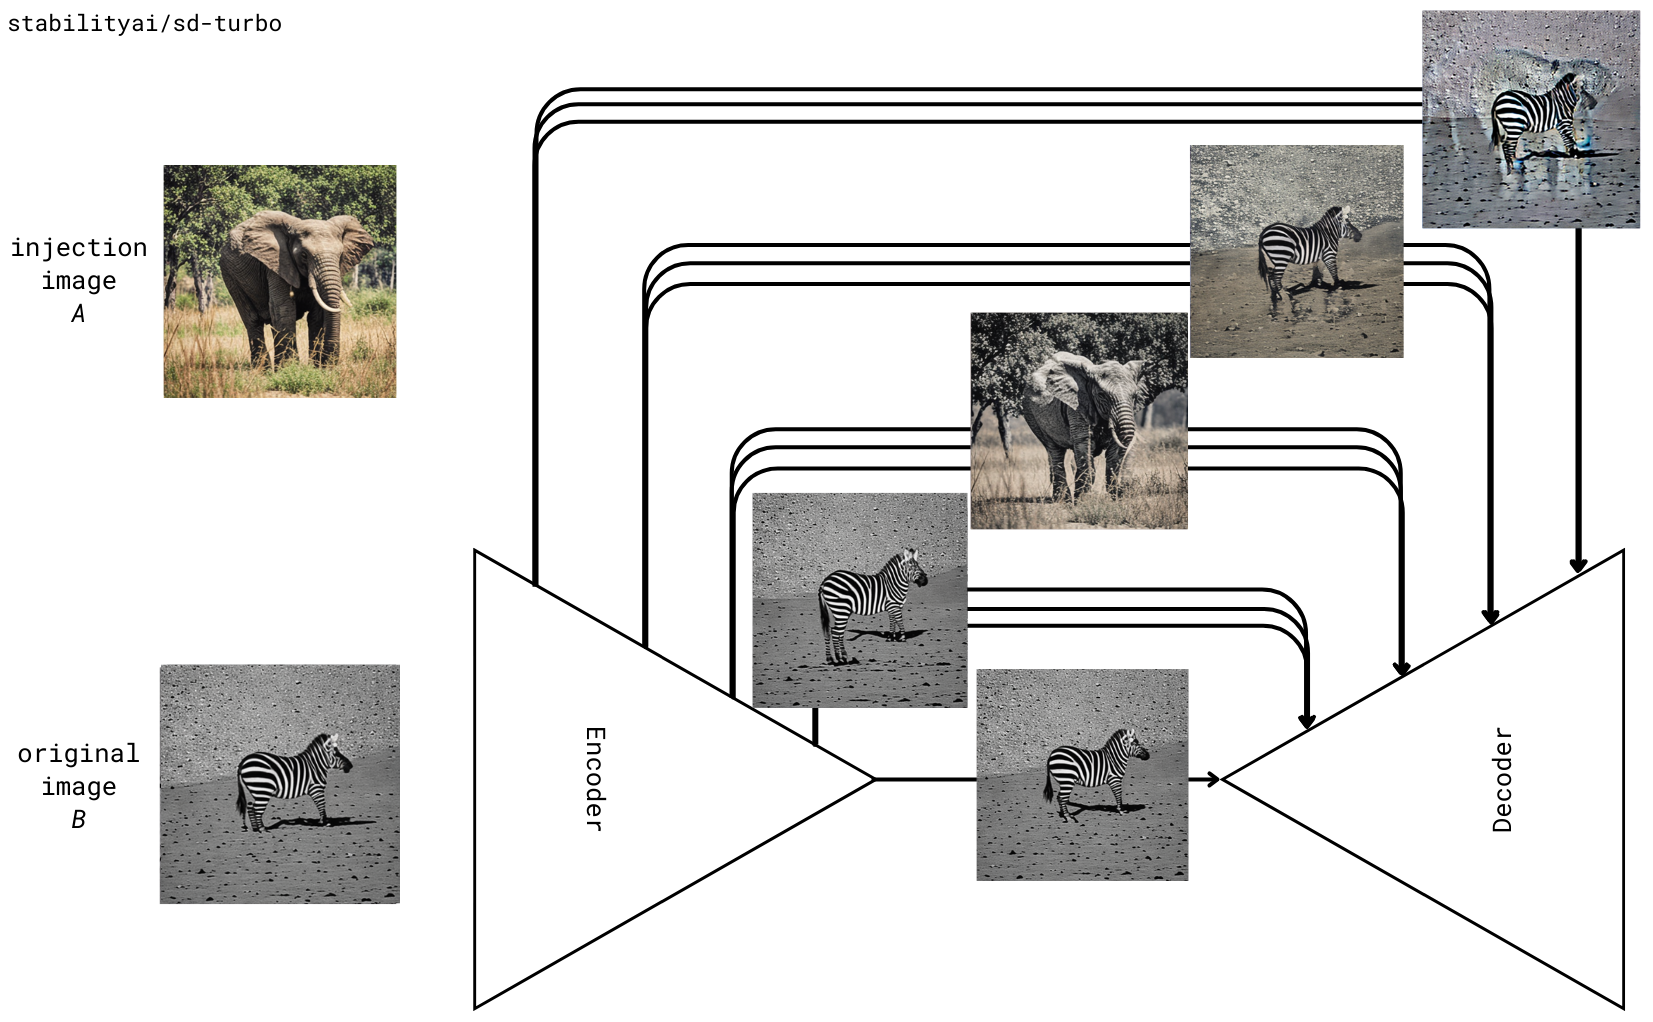}
\caption{Visualization of SkipInject effect on v2, v2.1, v2.1 Turbo. As visible in the figure, these three models have very similar effects. The content representation passes almost exclusively through the second group of skip connections, even in distilled Turbo versions.}
\label{fig:versions2}
\end{figure}

\begin{figure}[h]
\centering
\includegraphics[width=0.5\textwidth]{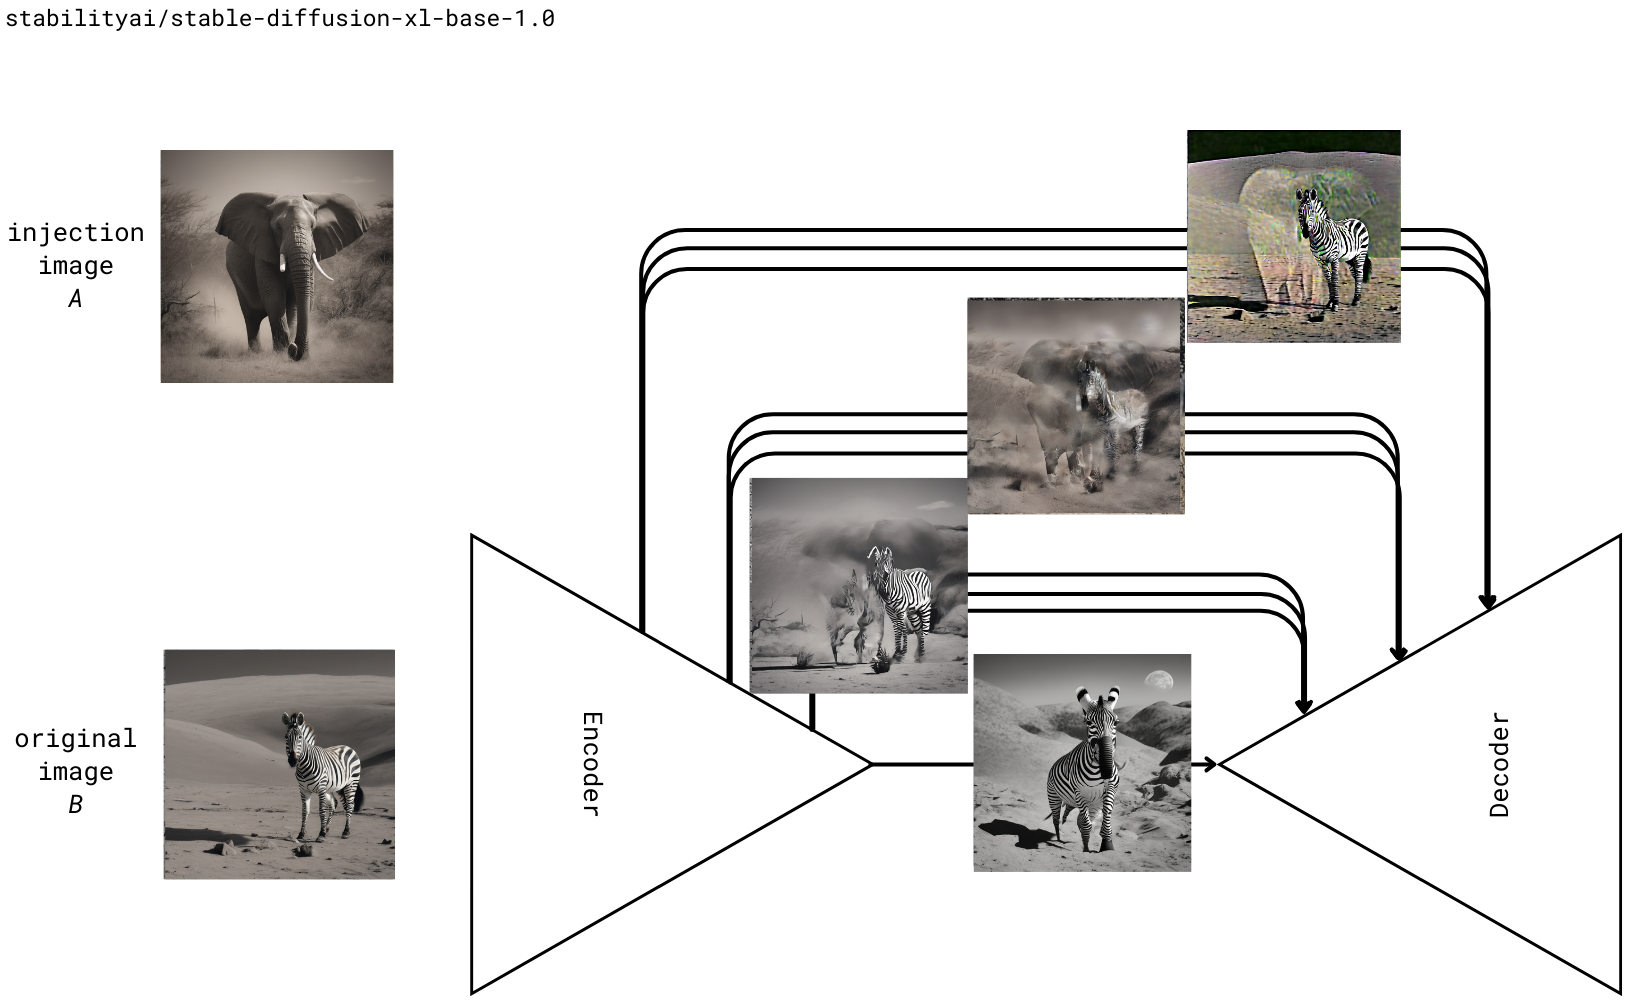}
\caption{Visualization of SkipInject effect on XL. As visible in the figure, the effect of the second group of skip connections is, as for v1.*, split between the \textit{h-space}, where the orientation and structure of the foreground are determined, and the second group of skips, determining the content of the background, without structure.}
\label{fig:versionsxl}
\end{figure}

In terms of architecture, the significant difference between Stable Diffusion v1.* and Stable Diffusion v2.* lies in the text embedding used for conditioning: the first versions use OpenAI's CLIP~\cite{radford_learning_2021}. In contrast, the second versions use OpenCLIP, trained on the publicly available LAION 2B dataset~\cite{schuhmann_laion-5b_2022}. Furthermore, Stable Diffusion v2.* uses a longer context length than v1.*, supporting a larger output size (from 512 to 768). The rest of the architecture remains unchanged. Stable Diffusion 2.*, despite producing higher resolution outputs, has seen a lower adoption, likely due to its incompatibility with the prompt engineered on versions 1.*\cite{noauthor_stable_2022}. 

Our analysis shows that the earlier versions put a much higher weight on the \textit{h-space}, indicating an evolution in the representations learned by these models. Given that most of the architecture remains unchanged, we can hypothesize that the CLIP embeddings cause the difference.

Stable Diffusion XL~\cite{podell_sdxl_2023} is the last UNet-based model released by StabilityAI. This model is about 4x larger than the previous Stable Diffusions and comprises base and refiner models. This section considers the base model responsible for generating the overall image. As visible in \cref{fig:versionsxl}, this model only features three downsampling blocks, with seldom cross-attentions in the first blocks and a concentration of the attention modules before the bottleneck. This model accepts two conditioning embeddings, one from OpenAI's CLIP, as in v1.*, and one from OpenCLIP, a larger version than the one used in v2.*. Because of this dual prompt, Stable Diffusion XL allows broader expressivity and the desired compatibility with v1.*.

In \cref{fig:versionsxl}, we observe that, interestingly, Stable Diffusion XL behaves very similarly to v1.*. While the speculation on the importance of the CLIP version still seems plausible, this phenomenon requires much deeper investigation, possibly underscoring studies on Diffusion models as representation learners.

\section{Ablation studies on the hyperparameters}
In this section, we test different configurations of the hyperparameters to ablate on our findings reported in the section Analyses. In that section, we recommend an ending timestep $\geq 350$ (indicated in the field \textbf{Injection t.}) to show the background specified by the modification and an interplay of the alternation (here referred to as \textbf{Altern.}, indicating every how often the injected embedding is substituted in depth with the original one) and guidance on the injected embedding (here referred to as \textbf{Switch g.}) for an improved tradeoff between the ability to follow the semantic editing and the maintenance of the structure.

\begin{table}[]
\centering
\resizebox{0.5\textwidth}{!}{\begin{tabular}{|l|l|l|l|l|l|l|}
\hline
\textbf{Skip}  & \textbf{Injection t.} & \textbf{Switch g.} & \textbf{Altern.} & \textbf{CLIP}     & \textbf{DINO} & \textbf{LPIPS}          \\ \hline
l=4   & (0, 1000)           & None            & None        & 0.289          & 0.033                & 0.421          \\ \hline
l=4,5 & (0, 1000)           & None            & None        & 0.278          & \textbf{0.018}       & \textbf{0.291} \\ \hline
l=4   & (400, 900)          & None            & None        & 0.301          & 0.045                & 0.497          \\ \hline
l=4,5 & (400, 900)          & None            & None        & 0.291          & 0.029               & 0.375          \\ \hline
l=4   & (400, 900)          & 0.75            & None        & 0.306          & 0.060                & 0.560          \\ \hline
l=4,5 & (400, 900)          & 0.75            & None        & 0.296          & 0.041                & 0.456          \\ \hline
l=4   & (400, 900)          & 0.75            & 10          & \textbf{0.308} & 0.065                & 0.581          \\ \hline
l=4,5 & (400, 900)          & 0.75            & 10          & \textit{0.299}          & \textit{0.048}               & \textit{0.497}          \\ \hline
l=4   & (400, 900)          & 0.75            & 20          & \textbf{0.308} & 0.062                & 0.569          \\ \hline
l=4,5 & (400, 900)          & 0.75            & 20          & 0.297          & 0.045                & 0.476          \\ \hline
l=4   & (400, 900)          & 1.5             & None        & 0.297          & 0.039                & 0.460          \\ \hline
l=4,5 & (400, 900)          & 1.5             & None        & 0.284          & 0.024                & 0.341          \\ \hline
\end{tabular}}
\caption{Ablation results on \texttt{imnetr-fake-ti2i} dataset. The best scores are indicated with bold, while the one considered the best compromise in italics. The metric named CLIP indicates CLIP score (higher better), DINO is the DINO self-similarity (lower better, as for LPIPS). The lowest DINO and LPIPS are achieved by the standard model across all timesteps using skips l=4,5, while the interplay of switch guidance and alternation achieves the highest CLIP scores. We believe l=4,5, with both guidance and alternation, achieves the best tradeoff on this dataset.}
\label{tab:imnetr-fake-ti2i}
\end{table}

In the \cref{tab:imnetr-fake-ti2i} and \cref{tab:wild-ti2i-fake}, we show, respectively, the prompt-to-image results on ImageNet and Wild. While in \cref{tab:imnetr-ti2i-real} and \cref{tab:wild-ti2i-real}, we present the results on image-to-image. The results are obtained with 50 inference steps (and inversion steps), UniPCMultistepScheduler, output size (512,512,) and classifier-free guidance 7.5.

\begin{table}[]
\centering
\resizebox{0.5\textwidth}{!}{\begin{tabular}{|l|l|l|l|l|l|l|}
\hline
\textbf{Skip} & \textbf{Injection t.} & \textbf{Switch g.} & \textbf{Altern.} & \textbf{CLIP}  & \textbf{DINO}  & \textbf{LPIPS} \\ \hline
l=4           & (0, 1000)             & None               & None             & 0.303          & 0.063          & 0.523          \\ \hline
l=4,5         & (0, 1000)             & None               & None             & 0.268          & \textbf{0.036} & \textbf{0.341} \\ \hline
l=4           & (400, 900)            & None               & None             & 0.308          & 0.080          & 0.564          \\ \hline
l=4,5         & (400, 900)            & None               & None             & 0.294          & 0.062          & 0.441          \\ \hline
l=4           & (400, 900)            & 0.75               & None             & 0.313          & 0.093          & 0.593          \\ \hline
l=4,5         & (400, 900)            & 0.75               & None             & 0.302          & 0.070          & 0.495          \\ \hline
l=4           & (400, 900)            & 0.75               & 10               & \textbf{0.316} & 0.101          & 0.621          \\ \hline
l=4,5         & (400, 900)            & 0.75               & 10               & 0.307          & 0.080          & 0.532          \\ \hline
l=4           & (400, 900)            & 0.75               & 20               & 0.315          & 0.097          & 0.610          \\ \hline
l=4,5         & (400, 900)            & 0.75               & 20               & \textit{0.303}          & \textit{0.073}          & \textit{0.510}          \\ \hline
l=4           & (400, 900)            & 1.5                & None             & 0.305          & 0.077          & 0.542          \\ \hline
l=4,5         & (400, 900)            & 1.5                & None             & 0.286          & 0.056          & 0.413          \\ \hline
\end{tabular}}
\caption{Ablation results on \texttt{wild-ti2i-fake} dataset. Similarly to \cref{tab:imnetr-fake-ti2i}, the lowest DINO and LPIPS are achieved by the standard model across all timesteps using skips l=4,5. In contrast, the interplay of switch guidance and alternation achieves the highest CLIP scores. Differently from \cref{tab:imnetr-fake-ti2i}, the best tradeoff is achieved with an alternation every 20 instead of 10. A higher alternation indicates lower modulation as to how often the embedding of the original image is injected into the injection embedding in depth.}
\label{tab:wild-ti2i-fake}
\end{table}
\begin{figure}[h]
\centering
\includegraphics[width=0.5\textwidth]{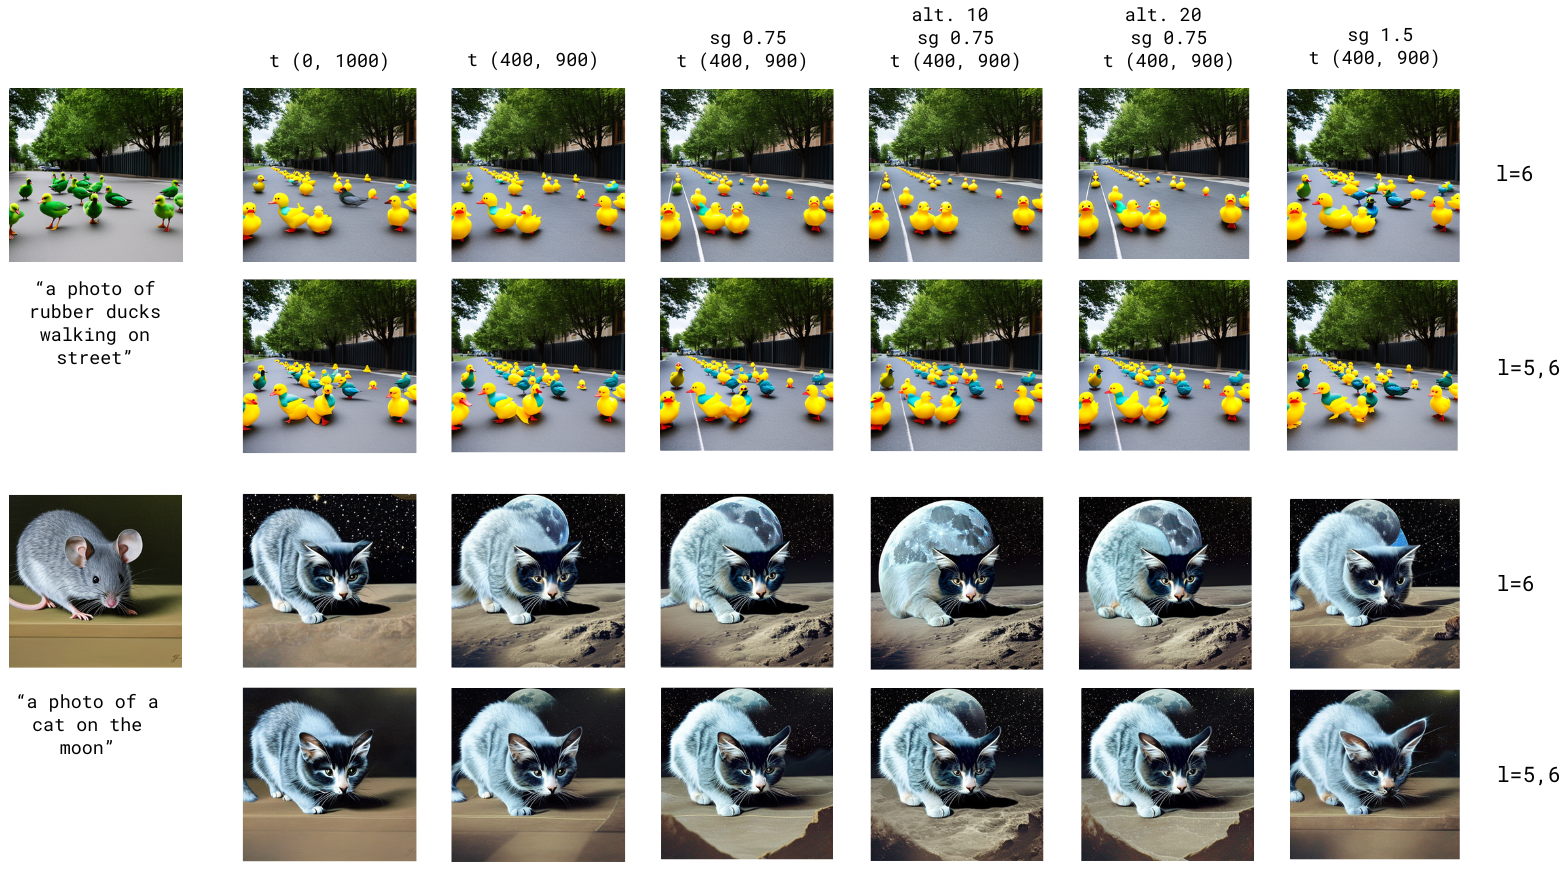}
\includegraphics[width=0.5\textwidth]{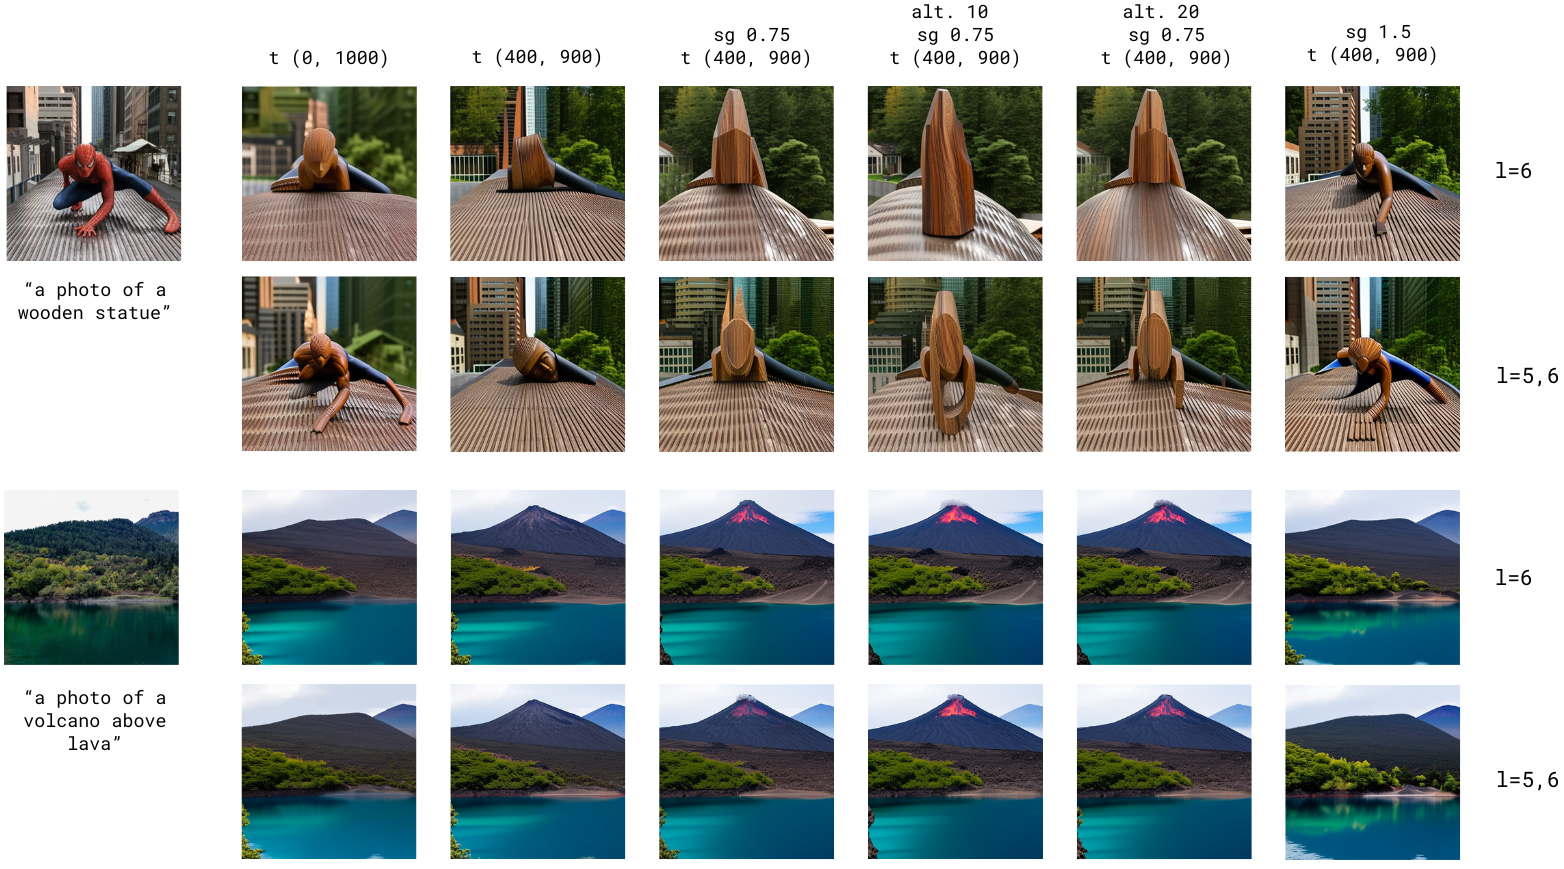}
\caption{Example results of text-guided image editing both on generated images (top) and inverted images (bottom) on different configurations of hyperparameters. We observe that, across most images, the base configuration already achieves reasonable results. When the background is specified (second image from the top), fewer injection timesteps contribute to forming the correct background. On the other side, the switch guidance and alternation strengthen the importance of the editing prompt, becoming particularly visible on the fourth image, whether the lava appears only when introducing switch guidance and the corresponding smoke with alternation.}
\label{fig:hyperparam}
\end{figure}

\begin{table}
\centering
\resizebox{0.5\textwidth}{!}{\begin{tabular}{|l|l|l|l|l|l|l|}
\hline
\textbf{Skip} & \textbf{Injection t.} & \textbf{Switch g.} & \textbf{Altern.} & \textbf{CLIP}  & \textbf{DINO}  & \textbf{LPIPS} \\ \hline
l=4           & (0, 1000)             & None               & None             & 0.288          & 0.059          & 0.524          \\ \hline
l=4,5         & (0, 1000)             & None               & None             & 0.275          & 0.047          & 0.494          \\ \hline
l=4           & (400, 900)            & None               & None             & 0.295          & 0.066          & 0.540          \\ \hline
l=4,5         & (400, 900)            & None               & None             & 0.287          & 0.052          & 0.505          \\ \hline
l=4           & (400, 900)            & 0.75               & None             & 0.302          & 0.078          & 0.567          \\ \hline
l=4,5         & (400, 900)            & 0.75               & None             & \textit{0.300}          & \textit{0.067}          & \textit{0.540}          \\ \hline
l=4           & (400, 900)            & 0.75               & 10               & \textbf{0.306} & 0.084          & 0.577          \\ \hline
l=4,5         & (400, 900)            & 0.75               & 10               & 0.301          & 0.073          & 0.556          \\ \hline
l=4           & (400, 900)            & 0.75               & 20               & 0.303          & 0.081          & 0.573          \\ \hline
l=4,5         & (400, 900)            & 0.75               & 20               & 0.300          & 0.069          & 0.546          \\ \hline
l=4           & (400, 900)            & 1.5                & None             & 0.290          & 0.056          & 0.515          \\ \hline
l=4,5         & (400, 900)            & 1.5                & None             & 0.278          & \textbf{0.046} & \textbf{0.483} \\ \hline
\end{tabular}}
\caption{Ablation results on \texttt{imnetr-ti2i-real} dataset. On this dataset, despite using fewer timesteps than the base configuration, the lowest DINO and LPIPS are achieved by switch guidance 1.5 using skips l=4,5.  Differently from \cref{tab:imnetr-fake-ti2i} and \cref{tab:wild-ti2i-fake}, the best tradeoff is achieved without any alternation on switch guidance 0.75.}
\label{tab:imnetr-ti2i-real}
\end{table}

\begin{table}[]
\centering
\resizebox{0.5\textwidth}{!}{\begin{tabular}{|l|l|l|l|l|l|l|}
\hline
\textbf{Skip} & \textbf{Injection t.} & \textbf{Switch g.} & \textbf{Altern.} & \textbf{CLIP}  & \textbf{DINO}  & \textbf{LPIPS} \\ \hline
l=4           & (0, 1000)             & None               & None             & 0.290          & 0.046          & 0.499          \\ \hline
l=4,5         & (0, 1000)             & None               & None             & 0.272          & \textbf{0.038} & 0.457          \\ \hline
l=4           & (400, 900)            & None               & None             & 0.298          & 0.054          & 0.513          \\ \hline
l=4,5         & (400, 900)            & None               & None             & 0.282          & 0.044          & 0.468          \\ \hline
l=4           & (400, 900)            & 0.75               & None             & 0.305          & 0.064          & 0.540          \\ \hline
l=4,5         & (400, 900)            & 0.75               & None             & 0.296          & 0.055          & 0.502          \\ \hline
l=4           & (400, 900)            & 0.75               & 10               & \textbf{0.307} & 0.068          & 0.549          \\ \hline
l=4,5         & (400, 900)            & 0.75               & 10               & \textit{0.302 }         & \textit{0.059 }         & \textit{0.515}          \\ \hline
l=4           & (400, 900)            & 0.75               & 20               & 0.305          & 0.066          & 0.544          \\ \hline
l=4,5         & (400, 900)            & 0.75               & 20               & 0.300          & 0.057          & 0.508          \\ \hline
l=4           & (400, 900)            & 1.5                & None             & 0.289          & 0.049          & 0.486          \\ \hline
l=4,5         & (400, 900)            & 1.5                & None             & 0.271          & 0.040          & \textbf{0.447} \\ \hline
\end{tabular}}
\caption{Ablation results on \texttt{wild-ti2i-real} dataset. On this dataset, the lowest DINO is achieved by the base configuration while the lowest LPIPS are achieved by switch guidance 1.5 using skips l=4,5.  Similarly to \cref{tab:imnetr-fake-ti2i}, the best tradeoff is obtained with alternation 10 and switch guidance 0.75.}
\label{tab:wild-ti2i-real}
\end{table}

Generally, we observe that an injection across all timesteps yields the most structural fidelity. Using switch guidance greater than one further decreases the DINO self-similarity and LPIPS. The highest prompt coherence is achieved by an interplay of switch guidance and alternation, with optimal results obtained on skips l=4,5. 

\begin{figure}[h]
\centering
\includegraphics[width=0.5\textwidth]{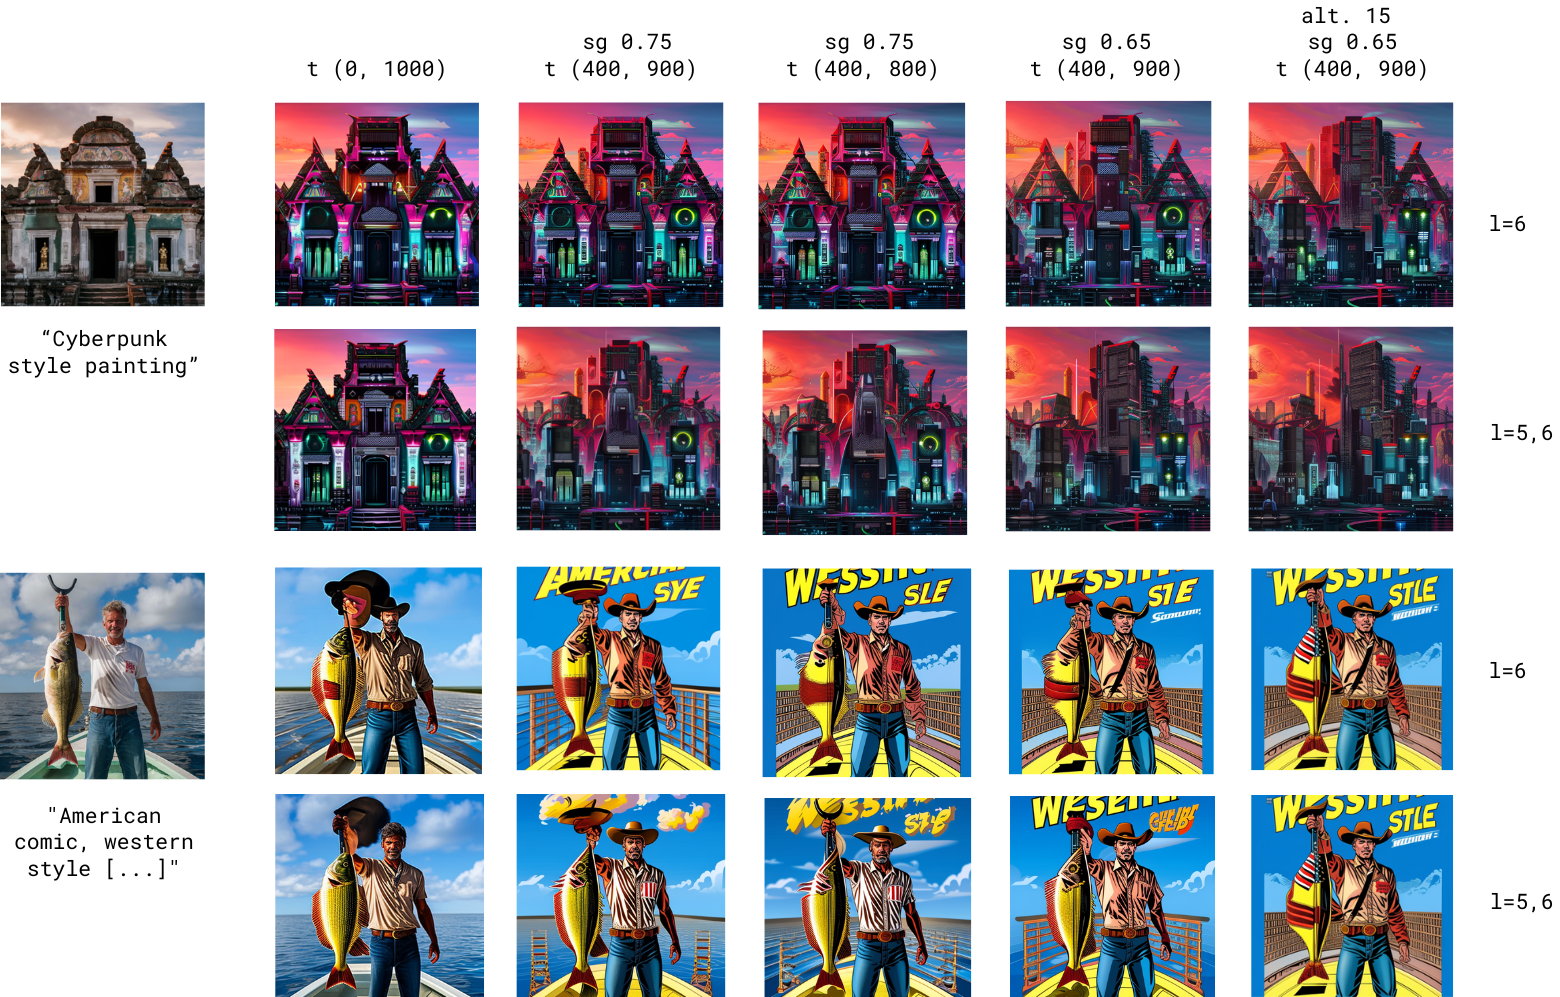}
\caption{Example results of style transfer on different configurations of hyperparameters. We observe that the standard configuration yields the most structurally sound results, but fails to transfer the style to the background. Using fewer timesteps and guidance or alternation increases the effect, also adjusting the subjects to be more coherent within that style.}
\label{fig:hyperparam_style}
\end{figure}

\centering
\begin{table}[]
\resizebox{0.5\textwidth}{!}{\begin{tabular}{|l|l|l|l|l|l|l|}
\hline
\textbf{Skip} & \textbf{Injection t.} & \textbf{Switch g.} & \textbf{Altern.} & \textbf{CLIP}  & \textbf{DINO}  & \textbf{LPIPS} \\ \hline
l=4           & (0, 1000)             & None               & None             & 0.217          & 0.036          & 0.481          \\ \hline
l=4,5         & (0, 1000)             & None               & None             & 0.186          & \textbf{0.025} & \textbf{0.398} \\ \hline
l=4           & (400, 900)            & 0.75               & None             & 0.263          & 0.054          & 0.580          \\ \hline
l=4,5         & (400, 900)            & 0.75               & None             & 0.236          & 0.037          & 0.483          \\ \hline
l=4           & (400, 800)            & 0.75               & None             & 0.270          & 0.060          & 0.608          \\ \hline
l=4,5         & (400, 800)            & 0.75               & None             & 0.248          & 0.041          & 0.515          \\ \hline
l=4           & (400, 900)            & 0.65               & None             & 0.271          & 0.062          & 0.613          \\ \hline
l=4,5         & (400, 900)            & 0.65               & None             & 0.252          & 0.044          & 0.528          \\ \hline
l=4           & (400, 900)            & 0.65               & 15               & \textbf{0.276} & 0.067          & 0.631          \\ \hline
l=4,5         & (400, 900)            & 0.65               & 15               & \textit{0.260 }         & \textit{0.050}          & \textit{0.559}          \\ \hline
\end{tabular}}
\caption{Ablation results on \texttt{artist} dataset. On this dataset, the lowest DINO and LPIPS are achieved by the base configuration using skips l=4,5, while the highest CLIP with switch guidance 0.65 and alternation 15 on skip 4. The l=4,5 (sg 0.65, alt 15) achieves the optimal configuration, lower in switch guidance and higher in alternation than text-based editing.}
\label{tab:artist}
\end{table}

\section{Examples on Turbo}
We show example results on Stable Diffusion Turbo.
\begin{figure}[h]
\centering
\includegraphics[width=0.5\textwidth]{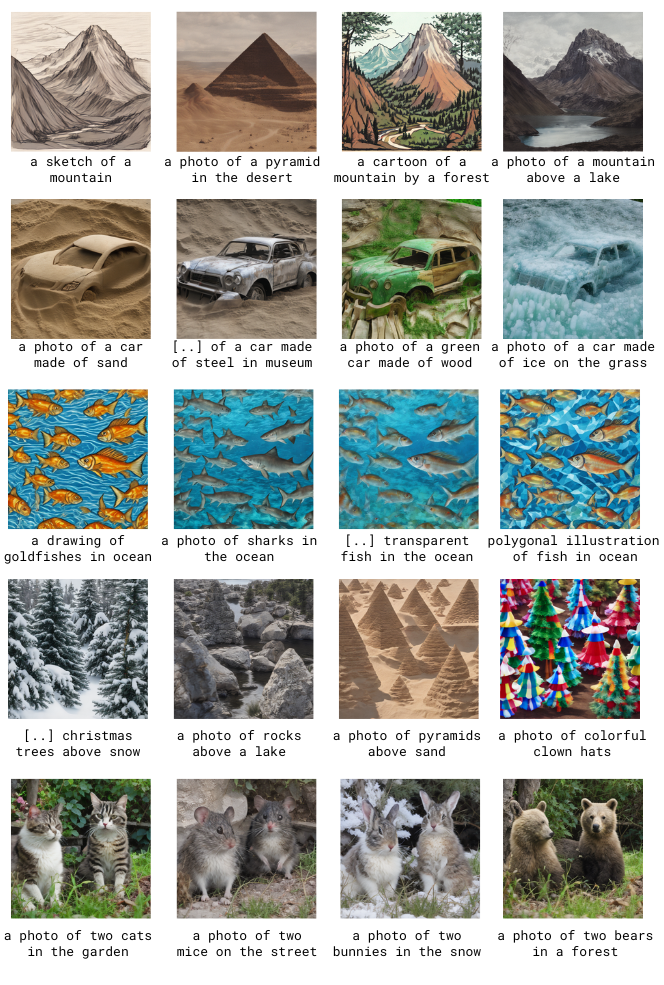}
\caption{Example results of text-based image editing using Stable Diffusion Turbo with 1 step inference on \texttt{wild-ti2i-fake}. The modifications obtained are coherent and cohesive, obtaining radical changes and maintaining the original structure. Compared to multi-step inference, the control over the background is more limited.}
\label{fig:turbo}
\end{figure}
